# Supplementary material for: From Self-Attention to Markov Models: Unveiling the Dynamics of Generative Transformers
Source: arXiv:2402.13512 source file (2024-02-21)
Supplement: Supplementary file 1 [file mapping_proof.tex]

\section{Proof of mapping between attention model and transition matrix}
\begin{theorem}\label{thm-mapping}
    For any transition matrix $\Pb \in \R^{K \times K}$, there exists $\W \in \R^{d \times d}$ such that for any input $X \in \R^{T \times d}$:
    \begin{align}
        \P_{\text{FreqX}\odot \Pb}(\x_{T+1}|\X)= \Cb\X^{\top}\mathbb{S}(\X\W\bar \x)
    \end{align}
    where $\Cb\Eb^{\top} = \Ib_K$
\end{theorem}
\begin{theorem}(Simplified version)\label{thm-mapping-easy} Assuming that $K \leq d$, $\text{rank}(\Eb) = K$ and $\Cb\Eb^{\top} = \Ib_K$.
    For any probability vector $\bpi \in \R^{K}$ where $\pi_k > 0$ for any $k \in [K]$, there exists a $\W \in \R^{d \times d}$ such that for any input $X \in \R^{T \times d}$:
    \begin{align} \label{eq-mapping-easy}
        \P_{\text{FreqX}\odot \bpi}(\x_{T+1}|\X)= \Cb\X^{\top}\mathbb{S}(\X\W\bar \x)
    \end{align}
    where $k$-th term of \text{FreqX} corresponds to the frequency of token $\eb_k$ in $\X$. Conversely, for any finite $\W$, there exists one and only one probability vector $\bpi$, where $\pi_k > 0$ for any $k \in [K]$,  satisfying Eq.~\eqref{eq-mapping-easy} for any input $\X$. 
\end{theorem}
\begin{proof}(of Theorem \ref{thm-mapping-easy})
    We first prove that for any probability vector $\bpi$ defined in Theorem~\ref{thm-mapping-easy}, there exists a $\W$ satisfying the Eq.~\eqref{eq-mapping-easy} for any input $\X$.   
    Suppose $\X = \M\Eb$ where $\M \in \R^{T \times K}$ is a universal mapping matrix, which specifies the token index for each entry. Specifically, $M_{jk} = 
                \begin{cases}
                    1, & \x_j = \eb_k \\ 
                    0, & \x_j \neq \eb_k
                \end{cases}$ Note that $\M^{\top} \mathbf{1} = \nb$ 
    %             = \begin{bmatrix}
    %     n_1 \\
    %     n_2 \\ 
    %     \vdots \\ 
    %     n_K  \\
    % \end{bmatrix} \in \R^{K}$, 
    , where $n_k$ is the frequency of token $\eb_k$ in $\X$. Define a function $g: \R^{K} \to \R^{K}$ which normalizes the input to a probability vector, i.e., $g(\vb) = \frac{\vb}{\|\vb\|_1}$. For the left side of the equation:
    \begin{equation} \label{eq-mapping-easy-trans}
        \begin{split}
           \P_{\text{FreqX}\odot \bpi}(\x_{T+1}|\X) &= g(\text{FreqX}\odot \bpi) \\ 
    & =g(\M^{\top}\mathbf{1} \odot \bpi)\\ 
    % &= g(\diag{\M^{\top}\mathbf{1}} \bpi) \\ 
    % &= \frac{1}{\sum_{k \in [K] } n_k \pi_k}
    % \begin{bmatrix}
    %     n_1\pi_1 \\
    %     n_2\pi_2 \\ 
    %     \vdots \\ 
    %     n_K\pi_K  \\
    % \end{bmatrix} \\ 
    % & = \frac{\nb \odot \bpi}{\sum_{k \in [K] } n_k \pi_k} \\ 
    & = g({\nb \odot \bpi})
    \end{split}
    \end{equation}
    Let $\m = \exp(\X\W\xb) , \bmb = \exp(\Eb\W\xb)$, then for the right hand side we have:
    % , $\tilW \coloneqq \Eb\W\Eb^{\top} \in \R^{K \times K} \text{ and } \bb_k^{(K)} \in \R^{K}$ be a standard basis with $k$-th entry being $1$
    \begin{equation} \label{eq-mapping-easy-attn}
        \begin{split}
         \Cb\X^{\top}\mathbb{S}(\X\W\bar \x) &= \M^{\top}\mathbb{S}(\X\W\xb) \\ 
        &= \frac{\M^{\top} \m}{\|\m\|_1}
        % \begin{bmatrix}
        % m_1 \\
        % m_2 \\ 
        % \vdots \\ 
        % m_T  \\
        % \end{bmatrix} 
        \\ 
        &\stackrel{(a)}= \frac{\M^{\top} \m}{\| \nb \odot \bmb \|_1}
        % \begin{bmatrix}
        % m_1 \\
        % m_2 \\ 
        % \vdots \\ 
        % m_T  \\
        % \end{bmatrix} 
        \\ 
        &\stackrel{(b)}= \frac{\nb \odot \bmb}{\| \nb \odot \bmb\|_1}
        % \begin{bmatrix}
        % n_1 \mb_1 \\
        % n_2 \mb_2 \\ 
        % \vdots \\ 
        % n_K \mb_K  \\
        % \end{bmatrix} 
        \\ 
        &= g(\nb \odot \bmb)
        \end{split}
    \end{equation} 
    where (a) merges $\mb_k = m_{j}$ if $\eb_k = \x_j$ and (b) comes from the definition of $\M$. As a result, comparing Eq.~\eqref{eq-mapping-easy-trans} and~\eqref{eq-mapping-easy-attn}, it is sufficient to prove that for any given $\bpi$, there exists a solution $\W$ for the following problem:
    \begin{equation}
         \bpi =  \exp(\Eb\W\xb)
    \end{equation}
    It is equivalent to solving the following linear system:
    \begin{equation}
        \Eb\w = \dot \bpi
    \end{equation}
    where $\w = \W \xb, \dot \bpi = \log \bpi$.
    Since the rows of $\Eb$ are linearly independent, $\Eb$ is right invertible, implying that there exists at least one solution to the problem above. \\ Next, we prove the converse of the statement: For any finite $\W$, there exists one and only one probability vector $\bpi$ satisfying Eq.~\eqref{eq-mapping-easy} for any input $\X$. Let $\bpi_0 = \exp(\Eb\W\xb)$. Substituting it into Eq.~\eqref{eq-mapping-easy}, we can show that $\bpi_0$ satisfies the equation for any input $\X$. Lastly we prove that $\bpi_0$ is the only solution by contradiction. Suppose to the contrary that there exists two solutions $\bpi_1 \neq \bpi_0$ satisfying Eq.~\eqref{eq-mapping-easy} for any input $\X$. Let $T = K, \X = \Eb $. Then $\nb = \mathbf{1}_K$. Since \begin{align*}
        g(\nb \odot \bpi_0) = g(\nb \odot \bpi_1) \text{ and } \|\bpi_0\| = \|\bpi_1\| = 1
    \end{align*}
    We have $\bpi_0 = \bpi_1$, which leads to a contradiction. 
 \end{proof}
 \begin{corollary}
    Suppose we have $\Pb^{grd} \in \R^{K \times K}$ such that all of the transitions are non-zero and Assumption \ref{assump nonzero q} holds. Suppose we have $\data$ such that $\hat{\Pb}$ defined in \eqref{EmpRisk} has only non-zero elements and there exists $\hat{\W} \in \R^{d \times d}$ that minimizes \eqref{EmpRisk W} for this $\data$. Then, with respect to the mapping defined in Theorem \ref{thm-mapping-easy}, we have
    \begin{enumerate}[label=(\roman*)]
        \item $\Wh$ and $\hat{P}$ are equivalent.
        \item $\Pb^*$ and $\W^*$ defined in \eqref{PopRisk} and \eqref{PopRisk W} are equivalent.
    \end{enumerate}
 \end{corollary}
